# Supplementary material for: Optimization of Hybrid Power Plants: When Is a Detailed Electrolyzer Model Necessary?
Source: arXiv:2301.05310 source file (2023-04-16)
Supplement: Supplementary file 1 [file AppendixB.tex]

\onecolumn

\begin{center}
    \Huge{Optimization of Hybrid Power Plants:
When Is a Detailed Electrolyzer Model Necessary?}
\\
\vspace{0.5cm}
\normalsize
Manuel Tobias Baumhof, Enrica Raheli, Andrea Gloppen Johnsen, and Jalal Kazempour
\\
Department of Wind and Energy Systems, Technical University of Denmark, Kgs. Lyngby, Denmark\\ 
$\{$mtba, enrah, anglopj, jalal$\}$@dtu.dk 
\end{center}

%\appendix
\vspace{0.5cm}
\section{Online Companion}

The following companion is supplementary to the paper \textit{Optimization of Hybrid Power Plants: When Is a Detailed Electrolyzer Model Necessary?} and provides the mathematical formulations of the MILP models with only two states (namely On-Off and On-Standby) in Section \ref{AppB} and \ref{AppC}, respectively. These are simplified models compared to the one proposed in Section \ref{model} with three states of the electrolyzer. All nomenclature is defined in the main paper. 
\vspace{0.5cm}
\subsection{The Simplified MILP with On-Off States}

\label{AppB}

This Section provides the MILP where the on and off states of the electrolyzer are only modeled. 
%\vspace{-0.05cm}
% format the equation environment
%reset the counter
\setcounter{equation}{0}

\begin{align}
 \label{MILP1}
    \underset{\bf{\Omega}}{\rm{max}}  \quad & \sum_{t \in \mathcal{T}} p_t \lambda^{\rm{DA}}_t + d_t \lambda^{\rm{h}} - z^{\rm{su}}_t \lambda^{\rm{su}} \\
%\text{Constraints}  \eqref{eq:start_1}, \eqref{eq:hy}-\eqref{eq:s_min}, \eqref{eq:stor_1}-\eqref{eq:demand}, \\
    \textrm{s.t.}  \quad & p_t = P^{\rm{w}}_t - p^{\rm{e}}_t - p^{\rm{c}}_t & \forall~ & t \in \mathcal{T},\\ 
    & p^{\rm{e}}_t  \leq C^{\rm{e}} z^{\rm{oo}}_t & \forall~ & t \in \mathcal{T}, \\
    & p^{\rm{e}}_t \geq P^{\rm{min}} z^{\rm{oo}}_t& \forall~ & t \in \mathcal{T},\\
    & z^{\rm{su}}_t \geq z^{\rm{oo}}_t - z^{\rm{oo}}_{t-1} & \forall~ & t \in \mathcal{T} \setminus \{1\} ,\\
    & z^{\rm{su}}_{t=1} = 0,  \\
    & h_t = \sum_{s \in \mathcal{S}} (A_s \hat{p}^{\rm{e}}_{ts} + B_s z^{\rm{h}}_{ts})& \forall~ & t \in \mathcal{T}, \\
    & \underline{P}_s  z^{\rm{h}}_{ts} \leq \hat{p}^{\rm{e}}_{ts} \leq  \overline{P}_s  z^{\rm{h}}_{ts} & \forall~ &  t \in \mathcal{T}, s \in \mathcal{S}, \\
    & z^{\rm{oo}}_t = \sum_{s \in \mathcal{S}} z^{\rm{h}}_{ts}  &\quad\forall~ & t \in \mathcal{T},\\
    & p^{\rm{e}}_t = \sum_{s \in \mathcal{S}} \hat{p}^{\rm{e}}_{ts} & \forall~ & t \in \mathcal{T} ,\\
    & h_t = h^{\rm{d}}_t + s^{\rm{in}}_t & \forall~ & t \in \mathcal{T}, \\
    & d_t = h^{\rm{d}}_t + s^{\rm{out}}_t & \forall~ & t \in \mathcal{T}, \\
    & s^{\rm{out}}_t \leq S^{\rm{out}} & \forall~ & t \in \mathcal{T}, \\
    & p^{\rm{c}}_t = K^{\rm{c}} s^{\rm{in}}_t & \forall~ & t \in \mathcal{T},\\
    & s_{t=1} = S^{\rm{ini}} + s^{\rm{in}}_{t=1} - s^{\rm{out}}_{t=1}, &  \\
    & s_t = s_{t-1} + s^{\rm{in}}_t - s^{\rm{out}}_t & \forall~ & t \in \mathcal{T} \setminus \{1\}, \\
    & s_t \leq C^{\rm{s}} & \forall~ & t \in \mathcal{T}, \\
    & \sum_{t \in \mathcal{H}_n} d_{t} \geq D_n^{\rm{min}} & \forall~ & n \in \{1, ..., N\}, \\
    %&\eqref{eq:start_1}, \eqref{eq:hy}-\eqref{eq:s_min}, \eqref{eq:stor_1}-\eqref{eq:demand}, \\
    &  d_t,  h_t, h^{\rm{d}}_t, p_t, p^{\rm{c}}_t, \hat{p}^{\rm{e}}_{ts},   s_t, s^{\rm{in}}_t, s^{\rm{out}}_t \in \mathbb{R}^+, &&\\
    & z^{\rm{su}}_t, z^{\rm{h}}_{ts}, z^{\rm{oo}}_t \in \{0,1\}, &&\\
    & \Omega = \{d_t,  h_t, h^{\rm{d}}_t, p_t, p^{\rm{c}}_t, \hat{p}^{\rm{e}}_{ts}, s^{\rm{in}}_t,   s^{\rm{out}}_t, z^{\rm{su}}_t, z^{\rm{h}}_{ts}, z^{\rm{oo}}_t \} .&&
\end{align}
