# Supplementary material for: Optimization of Hybrid Power Plants: When Is a Detailed Electrolyzer Model Necessary?
Source: arXiv:2301.05310 source file (2023-04-16)
Supplement: Supplementary file 2 [file AppendixC.tex]

\newpage

\subsection{The Simplified MILP  with On-Standby States} 
\label{AppC}

This Section presents the simplified MILP taking into account only the on and standby states of the electrolyzer.
%\vspace{-0.05cm}

\setcounter{equation}{0}

\begin{align}
    \underset{\Gamma}{\rm{max}} \quad & \sum_{t \in \mathcal{T}} p_t \lambda^{\rm{DA}}_t + d_t \lambda^{\rm{h}} - p^{\rm{in}}_t \lambda^{\rm{in}}_t\\
%\subsubsection{Constraints} \eqref{eq:market2},\eqref{eq:hy}-\eqref{eq:s_min}, \eqref{eq:stor_1}-\eqref{eq:demand},
    \textrm{s.t.}  \quad & p_t = P^{\rm{w}}_t + p^{\rm{in}}_t- p^{\rm{e}}_t - p^{\rm{c}}_t & \forall~ & t \in \mathcal{T},\\
    & p^{\rm{in}}_t \leq P^{\rm{sb}} (1-z^{\rm{os}}_t) & \forall~ & t \in \mathcal{T},\\
    & p^{\rm{e}}_t  \leq C^{\rm{e}} z^{\rm{os}}_t + P^{\rm{sb}} (1-z^{\rm{os}}_t) & \forall~ & t \in \mathcal{T}, \\
    & p^{\rm{e}}_t \geq P^{\rm{min}} z^{\rm{os}}_t + P^{\rm{sb}} (1-z^{\rm{os}}_t) & \forall~ & t \in \mathcal{T},\\
    & h_t = \sum_{s \in \mathcal{S}} (A_s \hat{p}^{\rm{e}}_{ts} + B_s z^{\rm{h}}_{ts})& \forall~ & t \in \mathcal{T},\\
    & \underline{P}_s  z^{\rm{h}}_{ts} \leq \hat{p}^{\rm{e}}_{ts} \leq  \overline{P}_s  z^{\rm{h}}_{ts} & \forall~ &  t \in \mathcal{T}, s \in \mathcal{S},\\
    & z^{\rm{os}}_t = \sum_{s \in \mathcal{S}} z^{\rm{h}}_{ts}  &\quad\forall~ & t \in \mathcal{T},\\
    & p^{\rm{e}}_t = \sum_{s \in \mathcal{S}} \hat{p}^{\rm{e}}_{ts} + P^{\rm{sb}} (1-z^{\rm{os}}_t) & \forall~ & t \in \mathcal{T},\\
    & h_t = h^{\rm{d}}_t + s^{\rm{in}}_t & \forall~ & t \in \mathcal{T}, \\
    & d_t = h^{\rm{d}}_t + s^{\rm{out}}_t & \forall~ & t \in \mathcal{T}, \\
    & s^{\rm{out}}_t \leq S^{\rm{out}} & \forall~ & t \in \mathcal{T}, \\
    & p^{\rm{c}}_t = K^{\rm{c}} s^{\rm{in}}_t & \forall~ & t \in \mathcal{T}, \\
    & s_{t=1} = S^{\rm{ini}} + s^{\rm{in}}_{t=1} - s^{\rm{out}}_{t=1} &  \\
    & s_t = s_{t-1} + s^{\rm{in}}_t - s^{\rm{out}}_t & \forall~ & t \in \mathcal{T} \setminus \{1\}, \\
    & s_t \leq C^{\rm{s}} & \forall~ & t \in \mathcal{T},\\
    & \sum_{t \in \mathcal{H}_n} d_{t} \geq D_n^{\rm{min}} & \forall~ & n \in \{1, ..., N\}, \\
   %& \eqref{eq:market2},\eqref{eq:hy}-\eqref{eq:s_min}, \eqref{eq:stor_1}-\eqref{eq:demand}, \\
    &  d_t,  h_t, h^{\rm{d}}_t, p_t, p^{\rm{c}}_t, p^{\rm{in}}_t, \hat{p}^{\rm{e}}_{ts},   s_t, s^{\rm{in}}_t, s^{\rm{out}}_t \in \mathbb{R}^+, \\
    & z^{\rm{h}}_{ts}, z^{\rm{os}}_t \in \{0,1\}, \\
    & \Gamma = \{d_t,  h_t, h^{\rm{d}}_t, p_t, p^{\rm{c}}_t, p^{\rm{in}}_t, \hat{p}^{\rm{e}}_{ts}, s^{\rm{in}}_t,  s_t,  s^{\rm{out}}_t, z^{\rm{su}}_t, z^{\rm{os}}_t \}.
\end{align}
